# Supplementary material for: CE-LoRA: Computation-Efficient LoRA Fine-Tuning for Language Models
Source: arXiv:2502.01378 source file (2025-02-03)
Supplement: Supplementary file 1 [file delta_experiment_settings.tex]

% \section{Additional Experiments}\label{app:delta}

% \textbf{Empirical justification of Assumption \ref{asp:contractive}. } In order to justify \eqref{eq:asp-ecgk}, we conduct experiments on language model fine-tuning tasks on \cgd{[XXX]} model using COLA, RTE and MRPC datasets, three tasks in the GLUE benchmark. In these experiments, we alternatively calculate one iteration of full gradient AdamW and one epoch of random gradient AdamW, each with a learning rate of \texttt{1e-5} for a total of 80 cycles. We apply a rank of 64 for both LoRA and double-LoRA in CeLoRA, and apply a compression rate of $p_{\mathrm{FFN}}=0.9$ and $p_{\mathrm{MHA}}=0.4$. We calculate the relative error $\|\mathbb{E}_{\xi^k\sim\mathcal{D}}[C(x^k;\xi^k)]-\nabla f(x^k)\|^2/\|\nabla f(x^k)\|^2$ for every full-gradient step, as illustrated in Fig.~\ref{fig:ecgk}, where all relative errors are below 1.


% \begin{figure}
%     \centering
%     \begin{minipage}{0.33\textwidth}
%         \includegraphics[width=\textwidth]{figures/histogram_cola_delta_fullgrad.png}
%     \end{minipage}
%     \begin{minipage}{0.33\textwidth}
%         \includegraphics[width=\textwidth]{figures/histogram_mrpc_delta_fullgrad.png}
%     \end{minipage}\begin{minipage}{0.33\textwidth}
%         \includegraphics[width=\textwidth]{figures/histogram_rte_delta_fullgrad.png}
%     \end{minipage}
%     \caption{Relative errors on COLA (left), MRPC (middle) and RTE (right).}
%     \label{fig:ecgk}
% \end{figure}
% The experiment selects three tasks in GLUE(COLA,RTE,MRPC) for testing. For full batch gradient descent, the experiment alternately uses one full gradient descent and one epoch of random gradient descent for training, calculates the relative error of the LoRA model and CeLoRA model for each full gradient descent, and performs a total of 80 cycles. For the stochastic gradient descent , the experiment train for 1 epoch per task and calculate the relative error every 10 iterations. The LoRA rank is 64, the CeLoRA Double LoRA method rank is 64, the MLP sampling ratio is 0.9, and the MHA sampling ratio is 0.4, We use google/gemma-2b as experiment model and the optimizer is AdamW, learning rate is 1e-5.

% \textbf{Ablation study for Double LoRA}
